# Supplementary material for: Content Filtering with Inattentive Information Consumers
Source: arXiv:2205.14060 source file (2023-12-20)
Supplement: Supplementary file 1 [file appendix_recovered.tex]

\section{Appendix}

We begin by applying the results of \cite{mm} to determine the
consumer's best response.  Much of the proceeding content will follow
directly.

\begin{lem}[Consumer's Best Response]
\label{lem:cbr}
  The consumer's unique best response to $\mixstrfil$ is
\begin{align}
  \tilde{\pi_0}^* & = \frac{(1-\mathcal{P}_c)}{(1-\mathcal{P}_c) +
                    \mathcal{P}_{c}e^{-c_2 / \lambda}} \nonumber \\
                           %& = \frac{\mathcal{P}_{c}e^{-c_2 / \lambda}}{\mathcal{P}_{c}e^{-c_2 / \lambda}+ (1-\mathcal{P}_c)}  \\
  & \text {and } \nonumber \\
  \tilde{\pi_1}^* & = \frac{(1-\mathcal{P}_{c})e^{-c_1/\lambda}}{(1-\mathcal{P}_c) e^{-c_1/\lambda} + \mathcal{P}_ce^{b/\lambda}}                                \label{eqn:cbr}
                            %& = \frac{\mathcal{P}_{c}e^{b /
                            %\lambda}}{\mathcal{P}_{c}e^{b / \lambda}+
                            %(1-\mathcal{P}_c)e^{-c_1/\lambda}}
\end{align}
where
\begin{align}
  \mathcal{P}_c = \min\left(1, \max\left(0,
  \frac{e^{b/\lambda}(\qfunc(\mixstrfil)-1) +
  e^{-c_1/\lambda}(1-\qfunc(\mixstrfil)e^{-c_2/\lambda})}{(e^{-c_2/\lambda}-1)(e^{b/\lambda}
  - e^{-c_1/\lambda})}\right)\right).
  \label{eqn:maxmin}
\end{align}
Furthermore, if $\mathcal{P}_c\in(0,1)$, the unique consumer optimal
actions is $s_{\texttt{c}}^*(0) = 0$ and $s_{\texttt{c}}^*(1) = 1$. If
$\mathcal{P}_c\notin(0,1)$, the consumer's optimal action is to ignore
all content or accept all content and choose a non-informative but
costless information strategy (i.e.
$\tilde{\pi}_1^* = \tilde{pi}_2^*$).
\end{lem}

\begin{proof}
  Fix the filter's strategy.  The consumer's strategy only impacts
  payoffs if $a_{\texttt{f}}=1$ so it sufficies to examine the
  consumer's best response conditional on the filter forwarding
  content.  Conditional on $a_{\texttt{f}}=1$, the consumer's decision
  problem is equivalent to a discrete choice problem under rational
  inattention as in \cite{mm} with prior probability
  $\qfunc(\mixstrfil)$.  Applying equation 13 as well as the
  guarantees of uniquesness provided in \cite{mm} gives the claimed
  results.
\end{proof}

\begin{proof}[Proof of Lemma \ref{lem:belief-BR}]
The attacker's strategy choice only enters  equation \ref{eqn:cbr}
through the $\qfunc(\mixstrfil)$ terms.  Furthermore,
$\qfunc(\mixstrfil)$ uniquely pins down consumer best response.  
\end{proof}

\begin{proof}[Proof of Proposition \ref{prop:goalposts}]
  If $\qfunc(\mixstrfil)<\qL$, then $P_c$ in lemma \ref{lem:cbr}
  is $1$ so the consumer's optimal strategy is to
  accept all content and incur no information costs.  A symmetric
  argument holds for when $\qfunc(\mixstrfil)>\qH$. Prove the other
  direction by contrapositive.  Assume $\infoC(\mixsigma)\neq 0$, then
  the consumer's best response cannot be to either accept all content
  or reject all content since it can do that by incuring no
  information costs.  This non-degenerate case only happens if
  $q\in(\qL,\qH)$ by lemma \ref{lem:cbr}.
\end{proof}

\begin{proof}[Proof of Lemma \ref{lm:min-diff}]
   For a filter's mixed strategy $\mixstrfil$, let
  $\gamma_0$ and $\gamma_1$ be the filter's probability of blocking
  after observing $0$ and $1$ respectively.  Then
  \begin{align}
    \qfunc(\mixstrfil) = \frac{(\pi_0(1-\gamma_0) + (1-\pi_0)(1-\gamma_1))q}{(\pi_0(1-\gamma_0) + (1-\pi_0)(1-\gamma_1))q + (\pi_1(1-\gamma_0) + (1-\pi_1)(1-\gamma_1))(1-q)}
  \end{align}

Taking derivatives with respect to both $\gamma_0$ and $\gamma_1$
establish that as long as $\pi_0>\pi_1$, $\qfunc(\mixstrfil)$ is
decreasing in $\gamma_0$ and increasing in $\gamma_1$ and thus
$\qfunc(\cdot)$ is minimized when $\gamma_0=1$ and $\gamma_1=0$ which
corresponds to $\strdif$.
\end{proof}

\begin{proof}[Proof of Corollarly \ref{cor:scaff-regimes}]
  To prove (a), note that by lemma \ref{lm:min-diff} if
  $\qfunc(\strdif)>q_H$ then $\qfunc(\mixstrfil)>q_H$ for any
  $\mixstrfil$ and by lemma \ref{lem:cbr} the consumer's best
  response when $\qfunc(\cdot)>q_H$ is to always block and therefore
  always blocking is dominant. The proof of (b) is symmetric and (c)
  follows once again directly from equation \ref{eqn:maxmin} in lemma
  \ref{lem:cbr}.
\end{proof}

\begin{proof}[Proof of Corollary \ref{cor:scaff-VoT}]
  To prove (a), note that under $\blkprof$ payoffs are $-(1-q)c_1$ and
  do not depend on $\pi_0$ or $\pi_1$.  Under $\fwdprof$, payoffs are
  given by $\E_{X,\scon}\sbr{ u(\acon,1,X) - \infoC\sbr{\scon;X \mid
      \afil=1}}$ which does not depend on $\pi_0$ or $\pi_1$ directly
  nor through the consumer's optimal strategy since
  $\qfunc(\fwdprof)=q$ for any values of $\pi_0$ and $\pi_1$.
  Finally, if $\qfunc(\difprof)>q_H$, the consumer's dominant strategy
  is to block all content and payoffs are again $-(1-q)c_1$ and do not
  depend on $\pi_0$ and $\pi_1$.  To prove (b), recall that when
  $\qfunc(\difprof)<q_L$ the consumer's strategy under $\difprof$ is
  to accept all content and this payoffs are given by
  $(1-q)(\pi_1(-c_1)+(1-\pi_1)b) + q(1-\pi_0)(-c_2)$ of which taking
  the derivatives are straightforward.
  \end{proof}

\begin{proof}[Proof of Lemma \ref{lem:terms}]
  Let $\tilde{\pi}_0^*$ and $\tilde{\pi}_1^*$ represent the consumer's
  optimal attention strategy as given in lemma \ref{lem:cbr}.
  Then:
  \begin{align*}
    \hat{V}(\qfunc(\mixstrfil))  &= \qfunc(\mixstrfil) \left( 1-\pot \right)  \left( -c_2 \right)  + \left( 1-\qfunc(\mixstrfil) \right) \ptt   \left( -c_1 \right)  +
                 \left( 1-\qfunc(\mixstrfil) \right)  \left( 1-\ptt \right) b -
                 \nonumber \\
               & \lambda \bigg[
                -\mathcal{P}_c \log \left(\mathcal{P}_c \right)  -
                 \left( 1-\mathcal{P}_c \right) \log \left(
                 1-\mathcal{P}_c \right)  + \nonumber \\
              & \qfunc(\mixstrfil)   \big( \pot\log \left( \pot \right)  +
                 \left( 1-\pot \right)  \log \left( 1-\pot \right)
                \big)  + \nonumber \\ 
    &  \left( 1-\qfunc(\mixstrfil) \right)    \big( \ptt\log \left( \ptt \right)  +
      \left( 1-\ptt \right)  \log \left( 1-\ptt \right) \big) \bigg]
      \nonumber \\
    \nonumber \\
       &= \qfunc(\mixstrfil) \left( 1-\pot \right)  \left( -c_2 \right)  + \left(
         1-\qfunc(\mixstrfil) \right) \ptt   \left( -c_1 \right)  + 
         \left( 1-\qfunc(\mixstrfil) \right)  \left( 1-\ptt \right) b -\nonumber \\
               & \lambda \bigg[-\mathcal{P}_c \log \left(\mathcal{P}_c \right)  -
                 \left( 1-\mathcal{P}_c \right) \log \left(
                 1-\mathcal{P}_c \right)  + \nonumber \\
               & \qfunc(\mixstrfil)\pot\log\big(\frac{\pot}{1-\pot}\big) +
                 (1-\qfunc(\mixstrfil))\ptt\log\big(\frac{\ptt}{1-\ptt}\big)  + \nonumber \\
               & \log(1-\pot) + (1-\qfunc(\mixstrfil))\log(1-\ptt)\bigg]  \nonumber   
  \end{align*}
Plugging in optimal values of $\pot$ and $\ptt$ from lemma
\ref{lem:cbr} gives
\begin{align*}
     &= \qfunc(\mixstrfil) \left( 1-\pot \right)  \left( -c_2 \right)  + \left( 1-\qfunc(\mixstrfil) \right) \ptt   \left( -c_1 \right)  +
                 \left( 1-\qfunc(\mixstrfil) \right)  \left( 1-\ptt \right) b -
                 \nonumber \\
               & \lambda \bigg[
                -\mathcal{P}_c \log \left(\mathcal{P}_c \right)  -
                 \left( 1-\mathcal{P}_c \right) \log \left(
                 1-\mathcal{P}_c \right)  + \nonumber \\
  & \qfunc(\mixstrfil) \pot
    \log\big(\frac{1-\mathcal{P}_c}{\mathcal{P}_ce^{-c_2/\lambda}}\big)
    + (1-\qfunc(\mixstrfil))\ptt\log\big(\frac{(1-\mathcal{P}_c)
    e^{-c_1/\lambda}}{\mathcal{P}_ce^{b/\lambda}}\big)  + \nonumber \\
 & \qfunc(\mixstrfil)\log\big(\frac{\mathcal{P}_ce^{-c_2/\lambda}}{\mathcal{P}_ce^{-c_2/\lambda} +
  1-\mathcal{P}_c}\big)  + (1-
  \qfunc(\mixstrfil))\log\big(\frac{\mathcal{P}_ce^{b/\lambda}}{\mathcal{P}_ce^{b/\lambda}+
   (1-\mathcal{P}_c)e^{-c_1/\lambda}}\big)\bigg] \nonumber
\end{align*}
After separating the logs and recognizing that $1-\mathcal{P}_c =
\qfunc(\mixstrfil)\pot + (1-\qfunc(\mixstrfil))\ptt$ the above simplifies to
\begin{align*}
  & = -\lambda\bigg[-\qfunc(\mixstrfil)\log\big(\mathcal{P}_ce^{-c_2/\lambda} + 1-\mathcal{P}_c\big)  - (1-
  \qfunc(\mixstrfil))\log\big(\mathcal{P}_ce^{b/\lambda}+
    (1-\mathcal{P}_c)e^{-c_1/\lambda}\big)\bigg] \nonumber \\
  &= \lambda\bigg[\qfunc(\mixstrfil)\log\big(\frac{\mathcal{P}_ce^{-c_2/\lambda} + 1-\mathcal{P}_c}{\mathcal{P}_ce^{b/\lambda}+
    (1-\mathcal{P}_c)e^{-c_1/\lambda}}\big) + \log\big(\mathcal{P}_ce^{b/\lambda}+
    (1-\mathcal{P}_c)e^{-c_1/\lambda}\big) \bigg] \nonumber
\end{align*}
Plugging in for $\mathcal{P}_c$ from lemma \ref{lem:cbr}
yields
\begin{align}
  &= \lambda\left[\qfunc(\mixstrfil)\log\left(\frac{\qfunc(\mixstrfil)}{1-\qfunc(\mixstrfil)}\frac{1-e^{-c_2/\lambda}}{e^{b/\lambda} - e^{-c_1/\lambda}}\right) + \log\left(\frac{(1-\qfunc(\mixstrfil))(e^{b/\lambda} - e^{-(c_1+c_2)/\lambda})}{1-e^{-c_2/\lambda}}\right)\right]
\end{align}
Separting out the $\qfunc(\mixstrfil)$ terms from within the logs and substituting 
$\frac{e^{-b/\lambda}(1-q_L)}{e^{c_2/\lambda}q_L}$ for the first term
and $\frac{e^b}{1-q_L}$ for the second term gives the claimed result
in terms of $q_L$.  Making similar substitutions with $q_H$ gives the
second expression in the claimed result.
\end{proof}

% \begin{lem}\label{lem:dexpr}
%   When $s_1=s_1^*$, if $I^*>0$, then
%   \begin{align*}
%   \frac{\partial{V(\sigma^d)}}{\partial{\pi_1}} =
%     -q\left[(1-\tilde{q})\frac{\partial \hat{V}^*}{\partial \tilde{q}} + \hat{V}(\sigma^d)\right] \nonumber \\
%   \frac{\partial{V(\sigma^d)}}{\partial{\pi_2}} = (1-q)\left(-c_1 + \tilde{q} \frac{\partial \hat{V}(\sigma^d)}{\partial \tilde{q}} - \hat{V}(\sigma^d)\right)
%     % \$ where
%   % $\mathbb{E}[R^*] = \tilde{q}(1-\tilde{\pi}_1^*)(-c_2) +
%   %   (1-\tilde{q})\tilde{\pi}_2^* + (1-\tilde{q})(1-\tilde{\pi}_2^*)b
%   \end{align*}
%     %and
%   % $I^*$ is the information cost evaluated at the equilibrium attention
%   % strategy.
%  \end{lem}
%  \begin{proof}
%    By using the results of lemma \ref{lem:eqb}, we can write the
%    equilibrium expected utility as
%    \begin{align}
%      V(\sigma^d) = (1-q)\pi_2(-c_1) +  \bigg(q(1-\pi_1) + (1-q)(1-\pi_2)\bigg)\hat{V}(\sigma^d)
%    \end{align}
%    taking derivatives with respect to $\pi_1$ gives
%    \begin{align}
%       \frac{\partial V(\sigma^d)}{\partial \pi_1} = 
%      \bigg(q(1-\pi_1) + (1-q)(1-\pi_2)\bigg)\bigg(\frac{\partial
%      \tilde{q} }{\partial \pi_1}\frac{\partial \hat{V}(\sigma^d)}{\partial \tilde{q}}\bigg)
%       + \hat{V}(\sigma^d)(-q)
%    \end{align}
%    Noting that $\frac{\partial \tilde{q}}{\partial \pi_1} =
%    \frac{-q(1-\pi_2)(1-q)}{((1-\pi_1)q + (1-\pi_2)(1-q))^2} =
%    \frac{-q(1-\tilde{q})}{(1-\pi_1)q + (1-\pi_2)(1-q)}$ and plugging
%    in gives the claimed result.  Deriving the expression for
%    $\frac{\partial V^*}{\partial \pi_1}$ follows identically.
%  \end{proof}

We begin by deriving profile payoffs and then use those to prove the
main results in section \ref{sec:aligned}.  We proceed in a different
order than the paper's body.  First we prove social optimality in pure
strategy profiles, then we show that the socially optimal pure profile
is better than any mixed.  Then we prove the value of technology.

\begin{lem}[Profile Payoffs]
  \label{lem:payterm}
  If $q, \qfunc(\strdif) \in (\qL, \qH)$ then
  \begin{align}
    V(\fwdprof) &= \hat{V}(q) \nonumber \\
    V(\difprof) &= (1-q)(\pi_1(-c_1) + (1-\pi_1)b) -q(1-\pi_0)(c_2) +\lambda\beta \KL{\qfunc(\strdif)}{\qL} \nonumber
  \end{align}
\end{lem}

\begin{proof}
The equation for $V(\fwdprof)$ is a straightforward application of
lemma \ref{lem:terms} since $\afil=1$ with probability $1$.  The
expression for $V(\difprof)$ is given by
\begin{align}
  V(\difprof) &= \mathbb{E}\big[P(\afil=0)V(\difprof|\afil=0) + P(\afil=1)V(\difprof|\afil=1)\big] \nonumber \\
  &=  (1-q)\pi_1(-c_1) + \beta(\hat{V}(q(\strdif)))\\
  &= (1-q)\pi_1(-c_1) + \beta\big( (1-\qfunc(\strdif))b -\qfunc(\strdif)c_2 + \lambda \KL{\qfunc(\strdif)}{q_L}\big)\nonumber
\end{align}
where $\beta = (1-\pi_0)q + (1-\pi_1)(1-q)$ is the probability the
filter forwards.  Multiplying through by $\beta$ and plugging in
$\frac{(1-\pi_0)q}{(1-\pi_0)q+(1-\pi_1)(1-q)}$ for $\qfunc(\strdif)$
and rearranging gives the claimed result.    
\end{proof}

% \begin{proof}[Proof of Proposition \ref{prop:aligned-best-eq}].

%   (This is a non-trivial proof because the filter's mixing
%   probabilities enter non-linearly into payoffs since it impacts the
%   information costs through the consumer's prior.  Therefore, standard
%   arguments regarding mixed strategies (even when incentives are
%   completely aligned) do not apply.  )

  % First note that $V(\difprof)$ and $V(\fwdprof)$ are lower bounded by
  % $V(\blkprof)$ since the consumer can always reject all content.  It
  % suffices to show that no mixed strategy equilibrium profile does
  % better than the maximum of $V(\difprof)$ and $V(\fwdprof)$.
  % % Specifically, since this is a game of common interest, if no mixed
  % % strategy does better than the greater of $V(\difprof)$ and
  % % $V(\fwdprof)$, than the profile yielding the higher payoff is a
  % % socially optimal equilibrium.
  % Lemma \ref{lem:cbr} already established that the consumer's best
  % response is unique so any mixed strategy equilibrium is one in which
  % only the filter mixes.

\begin{proof}[Proof of Proposition \ref{prop:diff}]
  Consider the parameter regimes separately:
  \begin{enumerate}
    \item If $q>q_H$, the consumer's best response under $\fwdprof$ is
      to block everything and earn $V(\blkprof)$.  This is a lower
      bound for $V(\difprof)$ since the consumer can always
      block everything and thus $V(\difprof)\geq
      V(\fwdprof)=V(\blkprof)$.  
    \item If $q_L<\qfunc(\difprof)<q<q_H$ then
      by lemma \ref{lem:payterm}
      \begin{align}
        &V(\difprof) - V(\fwdprof) > 0\implies \nonumber \\
        &(1-q)\pi_1(-c_1) + \beta\big( (1-\qfunc(\strdif))b -\tilde{q}c_2 + \lambda \KL{\qfunc(\strdif)}{q_L}\big)>(1-q)b -qc_2 + \lambda \KL{q}{q_L}
    % & \iff (1-p)\pi_1(-c_1) + \beta \lambda\left[\tilde{q}\log\left(\frac{\tilde{q}}{1-\tilde{q}}\frac{1-e^{-c_2/\lambda}}{e^{b/\lambda} - e^{-c_1/\lambda}}\right) + \log\left(\frac{(1-\tilde{q})(e^{b/\lambda} - e^{-(c_1+c_2)/\lambda})}{1-e^{-c_2/\lambda}}\right)\right] > \nonumber \\
    %               &\lambda\left[q\log\left(\frac{q}{1-q}\frac{1-e^{-c_2/\lambda}}{e^{b/\lambda} - e^{-c_1/\lambda}}\right) + \log\left(\frac{(1-q)(e^{b/\lambda} - e^{-(c_1+c_2)/\lambda})}{1-e^{-c_2/\lambda}}\right)\right]. \nonumber
                  % &\lambda \left[-\beta H(\tilde{q}) + H(q) +(\tilde{q}-q)\log(A)\right]>(1-q)\pi_2c_1 \nonumber \\
                  %  & \text{where}\;\;\;\;  A=\frac{1-e^{-c_2/\lambda}}{e^{b/\lambda} - e^{-c_1/\lambda}} \nonumber 
  \end{align}
  Rearranging terms gives the claimed result.  
  % \begin{align}
  %   &\lambda\left[H(X) - \beta H(X|a_{\texttt{f}}=1, s_{\texttt{f}}=\bar{s}_{\texttt{f}}) +\pi_0q\log\left(\frac{e^{b/\lambda}- e^{-c_1/\lambda}}{e^{b/\lambda} -e^{-(c_1+c_2)/\lambda}}\right) + \pi_1(1-q)\log\left(\frac{1-e^{-c_2/\lambda}}{e^{b/\lambda} -e^{-(c_1+c_2)/\lambda}}\right)\right] > \nonumber \\
  %   &(1-q)\pi_1c_1 \nonumber
  % \end{align}
  % Finally, noting that $\frac{1-e^{-c_2/\lambda}}{e^{b/\lambda}
  %   -e^{-(c_1+c_2)/\lambda}}=e^{-b/\lambda}(1-q_L)$ and rearranging
  % terms gives the claimed result.
    \item In this regime, the consumer's best response under
      $\difprof$ is to accept all content.  It's payoff under
      $\fwdprof$ is given by lemma \ref{lem:terms}. Therefore
      \begin{align}
        &V(\difprof) - V(\fwdprof) > 0\implies \nonumber \\
        & -q(1-\pi_0)c_2 +(1-q)\big(\pi_1(-c_1) + (1-\pi_1)b\big) >(1-q)b -qc_2 + \lambda D_{KL}(q||q_L) \nonumber
      \end{align}
       and rearranging terms once again gives the claimed result.  
    \item In this regime, the consumer accepts all content regardless
      of filter strategy and thus
      \begin{align}
        &V(\difprof) - V(\fwdprof) > 0\implies \nonumber \\
        & -q(1-\pi_0)c_2 +(1-q)\big(\pi_1(-c_1) + (1-\pi_1)b\big) >(1-q)b -qc_2 
      \end{align}
      and once again rearranging terms gives the claimed result.
    \end{enumerate}
\end{proof}

% \begin{proof}[Proof of Proposition \ref{prop:aligned-best-eq}].
%   First note that $V(\difprof)$ and $V(\fwdprof)$ are lower bounded by
%   $V(\blkprof)$ since the consumer can always reject all content.  It
%   suffices to show that no mixed strategy profile does better than the
%   maximum of $V(\difprof)$ and $V(\fwdprof)$.  Specifically, since
%   this is a game of common interest, if no consumer-optimal mixed
%   strategy does better than the greater of $V(\difprof)$ and
%   $V(\fwdprof)$, than the profile yielding the higher payoff is an
%   equilibrium.  Lemma \ref{lem:cbr} already established that the
%   consumer's best response is unique so any mixed strategy equilibrium
%   is one in which only the filter mixes.

%   We will proceed by contradiction.  Assume the some $\mixstrfil$ is
%   an optimal mixed strategy in the interior.  Then the
%   game is equivalent to a new game where the
%   filter plays a differentiating strategy but its signal distribution
%   is given by $\pi_0(\gamma_1-\gamma_0)+\gamma_1$ and
%   $\pi_1(\gamma_1-\gamma_0)+\gamma_1$ where $\gamma_0,\gamma_1$ are
%   the filter's random probabilities of blocking at each information
%   set.  

\begin{lem}\label{lem:qhv}
  Let $\mixsigma^1$ and $\mixsigma^2$ be  consumer-optimal profiles where
  the filter plays a (possibly degenerate) mixed strategy
  $\mixstrfil^1$ and $\mixstrfil^2$, respectively.  If
  $\qL<q(\mixstrfil^1)<q(\mixstrfil^2)<\qH$ then $V(\mixsigma^1)>V(\mixsigma^2)$
  if and only if
  $\beta_1 \KL{q(\mixstrfil^1)}{\qH}-\beta_2\KL{q(\mixstrfil^2)}{\qH}>0$
  where the $\beta_i$  is the unconditional probability of the
  filter forwarding under $\mixstrfil^i$.
\end{lem}
\begin{proof}
  Under a mixed strategy $\mixsigma^i$, payoffs are equivalent to payoffs in another
  game where the filter's signal is governed by
  $\pi_0(\gamma^i)=\pi_0(\gamma^i_0-\gamma^i_1)+\gamma^i_1$ and
  $\pi_1(\gamma^i)=\pi_1(\gamma^i_0-\gamma^i_1)+\gamma^i_1$ and the filter
  plays a differentiating strategy.  Using the $\qH$ expression for
  $\hat{u}$ yields
      \begin{align}
        &V(\mixsigma^1) - V(\mixsigma^2) > 0\implies \nonumber \\
        &(1-q)\pi_1(\gamma^1)(-c_1) + \beta_1\big( -(1-\qfunc(\mixstrfil^1))c_1 + \lambda \KL{\qfunc(\mixstrfil^1)}{\qH}\big)> \nonumber \\
        &\;\;\;\;\;\;\;\;\;\;\;\;\;\;\; (1-q)\pi_1(\gamma^2)(-c_1) + \beta_2\big( -(1-\qfunc(\mixstrfil^2))c_1 + \lambda \KL{\qfunc(\mixstrfil^2)}{\qH}\big)
    % & \iff (1-p)\pi_1(-c_1) + \beta \lambda\left[\tilde{q}\log\left(\frac{\tilde{q}}{1-\tilde{q}}\frac{1-e^{-c_2/\lambda}}{e^{b/\lambda} - e^{-c_1/\lambda}}\right) + \log\left(\frac{(1-\tilde{q})(e^{b/\lambda} - e^{-(c_1+c_2)/\lambda})}{1-e^{-c_2/\lambda}}\right)\right] > \nonumber \\
    %               &\lambda\left[q\log\left(\frac{q}{1-q}\frac{1-e^{-c_2/\lambda}}{e^{b/\lambda} - e^{-c_1/\lambda}}\right) + \log\left(\frac{(1-q)(e^{b/\lambda} - e^{-(c_1+c_2)/\lambda})}{1-e^{-c_2/\lambda}}\right)\right]. \nonumber
                  % &\lambda \left[-\beta H(\tilde{q}) + H(q) +(\tilde{q}-q)\log(A)\right]>(1-q)\pi_2c_1 \nonumber \\
                  %  & \text{where}\;\;\;\;  A=\frac{1-e^{-c_2/\lambda}}{e^{b/\lambda} - e^{-c_1/\lambda}} \nonumber 
      \end{align}
      After multiplying through by the $\beta$ terms, The $c_1$ terms cancel thus proving the results.
    \end{proof}

    \begin{lem}\label{lem:qhv2}

      Let $\mixsigma$ be a consumer-optimal profile where the filter
      plays a (possibly degenerate) mixed strategy.  If
      $q(\strdif)<\qL\leq q(\mixstrfil)<\qH$ then
      $V(\difprof)>V(\mixsigma)$ if and only if
      $\Delta U^{\prime}>\beta_{\gamma}\KL{q(\mixsigma)}{\qH}$ and
      $\Delta U^{\prime}=(1-q)(1-\pi_1)(b+c_1) -q (1-\pi_0)c_2$
      where $\beta_{\gamma}$ is the unconditional probability of the
      filter forwarding under $\mixstrfil$.
  
  % If $\qdif<\qL<q<\qH$ then $V(\difprof)>V(\fwdprof)$ if and only if
  % $\Delta U^{\prime}>\KL{q}{\qH}$ where $\Delta
  % U^{\prime}=(1-q)(1-\pi_1)(b+c_1) -q (1-\pi_0)c_2$
\end{lem}
\begin{proof}
  Using the $\qH$ expression for $\hat{u}$ yields
       \begin{align}
         V(\difprof) - V(\mixsigma) > 0\implies \nonumber \\
         (1-q)(\pi_1(-c_1)+(1-\pi_1)b) -qc_2(1-\pi_0) >-(1-q)\pi_1^{\gamma}c_1 + \beta_\gamma (-(1-q(\mixstrfil))c_1 + \lambda \KL{q}{q_H})
  %   % & \iff (1-p)\pi_1(-c_1) + \beta \lambda\left[\tilde{q}\log\left(\frac{\tilde{q}}{1-\tilde{q}}\frac{1-e^{-c_2/\lambda}}{e^{b/\lambda} - e^{-c_1/\lambda}}\right) + \log\left(\frac{(1-\tilde{q})(e^{b/\lambda} - e^{-(c_1+c_2)/\lambda})}{1-e^{-c_2/\lambda}}\right)\right] > \nonumber \\
  %   %               &\lambda\left[q\log\left(\frac{q}{1-q}\frac{1-e^{-c_2/\lambda}}{e^{b/\lambda} - e^{-c_1/\lambda}}\right) + \log\left(\frac{(1-q)(e^{b/\lambda} - e^{-(c_1+c_2)/\lambda})}{1-e^{-c_2/\lambda}}\right)\right]. \nonumber
  %                 % &\lambda \left[-\beta H(\tilde{q}) + H(q) +(\tilde{q}-q)\log(A)\right]>(1-q)\pi_2c_1 \nonumber \\
  %                 %  & \text{where}\;\;\;\;  A=\frac{1-e^{-c_2/\lambda}}{e^{b/\lambda} - e^{-c_1/\lambda}} \nonumber 
       \end{align}
  %     Rearranging terms  proving the claim.
    where the $\pi_1^{\gamma}$ is as in lemma \ref{lem:qhv}.
    Rearranging the terms gives the claimed result.  
    \end{proof}

\begin{proof}[Proof of Proposition \ref{prop:aligned-best-eq}].      
  (This is a non-trivial proof because the filter's mixing
  probabilities enter non-linearly into payoffs since it impacts the
  information costs through the consumer's prior.  Therefore, standard
  arguments regarding mixed strategies (even when incentives are
  completely aligned) do not apply.)

  First note that $V(\difprof)$ and $V(\fwdprof)$ are lower bounded by
  $V(\blkprof)$ since the consumer can always reject all content.  It
  suffices to show that no mixed strategy profile does better than the
  maximum of $V(\difprof)$ and $V(\fwdprof)$.  Specifically, since
  this is a game of common interest, if no consumer-optimal mixed
  strategy does better than the greater of $V(\difprof)$ and
  $V(\fwdprof)$, than the profile yielding the higher payoff is the
  socially optimal equilibrium.  Lemma \ref{lem:cbr} already
  established that the consumer's best response is unique so any mixed
  strategy equilibrium is one in which only the filter mixes.

  Let $\mixstrfil$ be the filter's mixed strategy and assume the
  consumer best responds. Then the
  game is equivalent to a new game where the
  filter plays a differentiating strategy but its signal distribution
  is given by $\pi_0(\gamma_1-\gamma_0)+\gamma_1$ and
  $\pi_1(\gamma_1-\gamma_0)+\gamma_1$ where $\gamma_0,\gamma_1$ are
  the filter's random probabilities of blocking at each information
  set.  If $\gamma_0<\gamma_1$ then the filer is more likely to
  forward malicious content than clean content, which is a a weakly
  dominated strategy, so we can focus on the case where
  $\gamma_0>\gamma_1$.  This also implies that
  $q(\strdif)<q(\mixstrfil)<q$. 

  The case where $q(\mixstrfil)>\qH$ is trivial since the optimal
  payoff under that regime is $V(\blkprof)$, which is weakly dominated
  by any other pure strategy profile.  Furthermore when
  $q(\mixstrfil)\leq\qL$, the payoffs are linear in $\gamma_0$ and
  $\gamma_1$ and thus the filter would be better on the edge, which
  corresponds either to $\fwdprof$ or $\difprof$ or setting
  $q(\mixstrfil)=\qL$. which we will show is also not optimal.  

  %Without loss of generality, we can assume
    % $\gamma_1>\gamma_2$ which corresponds to the 
    % case where the filter is more likeliy to block malicious content
    % than clean.   

  Fix the filter's mixed strategy at $\mixstrfil$ such that
  $\qL\leq q(\mixstrfil)<\qH$.  Applying lemma \ref{lem:terms} means
  that the player's optimal payoff when the filter plays mixed
  strategy $\mixstrfil$ is given by
  $\beta_{\gamma}\lambda \KL{q(\mixstrfil)}{\qH}$ where
  $\beta_{\gamma}$ is the unconditional probability the filter
  forwards content.  Let
  $t=\frac{q-q(\mixstrfil)}{q-q(\strdif)}=1-\frac{\gamma_0}{\beta_{\gamma}}$
  such that $tq(\strdif) + (1-t)q = q(\mixstrfil)$.  Then by convexity
  of KL divergence
    \begin{align}
      \KL{q(\mixstrfil)}{\qH}<t \KL{q(\strdif)}{\qH} + (1-t)\KL{q}{\qH} \nonumber \\
      \rightarrow \gamma_0\big(\KL{q(\strdif)}{\qH} - \KL{q}{\qH}\big) < \beta_{\gamma}\KL{q(\strdif)}{\qH} - \beta_{\gamma}\KL{q(\mixstrfil}{\qH} \nonumber
    \end{align}
    writing the first $\beta_{\gamma}$ term as $\beta + \beta_{\gamma} - \beta$ and
    rearranging yields
    \begin{align}
      (\gamma_0+\beta - \beta_{\gamma})\KL{q(\strdif)}{\qH} - \gamma_0 \KL{q}{\qH}< \beta \KL{q(\strdif)}{\qH} - \beta_{\gamma}\KL{q(\mixstrfil)}{\qH} \nonumber
    \end{align}
    and recognizing that $\gamma_0+\beta -
    \beta_{\gamma}=(1+\gamma_0-\gamma_1)\beta$ the inequality can be
    written as 
\begin{align}
  (1+\gamma_0-\gamma_1)\beta \KL{q(\strdif)}{\qH} - \gamma_0 \KL{q}{\qH}< \beta \KL{q(\strdif)}{\qH} - \beta_{\gamma}\KL{q(\mixstrfil)}{\qH} \label{eq:nomix00} \\
  \rightarrow \gamma_0\big(\beta \KL{q(\strdif)}{\qH} -  \KL{q}{\qH}\big)< \beta \KL{q(\strdif)}{\qH} - \beta_{\gamma}\KL{q(\mixstrfil)}{\qH} \label{eq:nomix1}
\end{align}
where the second line follows because $1-\gamma_1>0$.

\textbf{Case 1:} Suppose $\qL\leq q(\strdif)<q<qH$: First, suppose
$V(\difprof)>V(\fwdprof)$, then by lemma \ref{lem:qhv} it suffices to
show that
$\beta \KL{q(\sfil)}{\qH}-\beta_{\gamma} \KL{q(\mixstrfil)}{\qH}>0$.
By lemma \ref{lem:qhv} the left hand side of equation \ref{eq:nomix1}
is positive so the right hand side must also be positive thus proving
the sufficient condition.  Now, suppose $V(\difprof)<V(\fwdprof)$,
then again by lemma \ref{lem:qhv} it suffices to show that
$\KL{q}{qH}-\beta_{\gamma} \KL{q(\mixstrfil)}{\qH}>0$.  This can be
accomplished by adding $\KL{q}{\qH}$ to each side and rearranging
\ref{eq:nomix1} to read
\begin{align}
  (\gamma_0-1)(\beta \KL{q(\strdif)}{\qH} -\KL{q}{\qH})< \KL{q}{\qH} - \beta_{\gamma}\KL{q(\mixstrfil)}{\qH}
\end{align}
and since by assumption $V(\difprof)<V(\fwdprof)$ both terms on the
left hand side are negative so the right hand side must be positive,
thus completing the proof.

\textbf{Case 2:} Suppose $q(\strdif)<\qL\leq q(\mixstrfil)$.  First
suppose $V(\difprof)>V(\fwdprof)$.  By lemma \ref{lem:qhv2} we must
show that $\delta U^{\prime}>\beta_{\gamma}\KL{q(\mixstrfil)}{\qH}$.
By applying lemma \ref{lem:qhv2}, $\delta U^{\prime}>\KL{q}{\qH}$ and
thus we can plug $\delta U^{\prime}$ into \ref{eq:nomix00} and
rearrange to obtain.
\begin{align}
  (\gamma_0 - \gamma_1)\beta \KL{q(\strdif)}{\qH} + \beta_{\gamma}\KL{q(\mixstrfil)}{\qH}<\gamma_0 \Delta U^{\prime} \label{eq:nomix2}
\end{align}
Since by assumption $\gamma_0>\gamma_1$, and $0\gamma_0<1$, expression
\ref{eq:nomix2} implies $\beta_{\gamma}\KL{q(\mixstrfil)}{\qH}< \Delta
U^{\prime}$, completing the proof.  

Finally, suppose $V(\difprof)<V(\fwdprof)$. Then it we must show that
show that $\KL{q}{\qH}>\beta_{\gamma}\KL{q(\mixstrfil)}{\qH}$ which we
can do by rearranging equation \ref{eq:nomix00} to be
\begin{align}
  (\gamma_0-\gamma_1)\beta \KL{q(\strdif)}{\qH} <  \gamma_0 \KL{q}{\qH} - \beta_{\gamma}\KL{q(\mixstrfil)}{\qH} \label{eq:nomixlast}
\end{align}
and since by assumption $(1<\gamma_0<\gamma_1)$, equation
\ref{eq:nomixlast} implies
$\KL{q}{\qH}>\beta_{\gamma}\KL{q(\mixstrfil)}{\qH}$.  This completes
the proof for all cases.  
  \end{proof}

\begin{proof}[Proof of Theorem \ref{thm:dvdp}]
  Part (a) and (b)  of theorem \ref{thm:dvdp}  follow directly from
  corollary \ref{cor:scaff-VoT}.  %  since in that regime the socially optimal profile is for the
  % filter to differentiate and the consumer to accept all content.
  To prove the third claim, using lemma \ref{lem:terms} socially
  optimal equilibrium payoffs can be expresed as
   \begin{align}
     V^* =  V(\fwdprof) &= (1-q)\pi_1(-c_1) + \beta\big(-(1-q(\strdif))c_1 +\lambda \KL{q(\strdif)}{q_H}\big) \nonumber \\
     &=(1-q)(-c_1) + \beta\lambda\KL{q(\strdif)}{q_H}
   \end{align}
   and taking the derivative with respect to $\pi_0$ and $\pi_1$ is
   then straightforward.  
   % \noindent Again, by using the expression for $\hat{V}(\sigma^d)$ in
   % lemma \ref{lem:terms}, it is straightforward to show that
   % \begin{align}
   % \frac{\partial \hat{V}(\sigma^d)}{\partial \tilde{q}} &= -\lambda \log\bigg(\frac{1-\tilde{q}}{\tilde{q}}\frac{e^{b/\lambda} - e^{-c_1/\lambda}}{1-e^{-c2/\lambda}}\bigg) \label{eq:dvbar}
   % \end{align}
   % Plugging equations \ref{eq:eut} and \ref{eq:dvbar} into equation \ref{eq:dpi1p} and
   % noting that $\frac{\partial \tilde{q}}{\partial \pi_0} =
   % \frac{-q(1-\pi_1)(1-q)}{((1-\pi_0)q + (1-\pi_1)(1-q))^2} =
   % \frac{-q(1-\tilde{q})}{(1-\pi_0)q + (1-\pi_1)(1-q)}$ gives the
   % claimed result.  Deriving the expression for 
   % $\frac{\partial V^*}{\partial \pi_1}$ follows identically.
 \end{proof}

 % \begin{proof}[Proof of Corollary \ref{cor:dderiv}]
 %   It is sufficient to show that $\nabla_{\mathbf{\pi}} V(\sigma^*)
 %   \not \propto  \nabla_{\mathbf{\pi}} \tilde{q}$.
 %   The expression for $\nabla_{\mathbf{\pi}} V^(\sigma^*)$ is given in
 %   proposition \ref{prop:dvdp} and
 %   $\nabla_{\mathbf{\pi}} \tilde{q}=(-\frac{q(1-\tilde{q})}{L},
 %   \frac{\tilde{q}(1-q)}{L})$ where $L= (1-\pi_0)q + (1-\pi_1)(1-q)$,
 %   which is not proportional to $\nabla_{\mathbf{\pi}} V^(\sigma^*)$
 %   almost everywhere.
 %   \end{proof}

 \begin{proof}[Proof of Lemma \ref{lem:nomixsemi}]
   The proof for the consumer is identical to the proof in the aligned
   case.  Now consider the filter.  Let $\mixsigma$ be a consumer
   optimal profile in which the filter mixes according to
   $\mixstrfil$.  % For it to be an equilibrium for the filter to
   % randomize at an information set, it must be indifferent between
   % forwarding content and blocking.  Therefore, any equilibrium
   % profile in which the filter blocks with positive probability at
   % both information sets achievs a payoff of $\Vfil(\blkprof)$ which
   % is a lower bound of $\Vfil(\difprof)$ and $\Vfil(\fwdprof)$.  The
   % profile where the filter blocks after reciving the signal that
   % content is clean and forwards after reciving the malicious signal
   % is a never-best response and is thus dominated.  Therefore, it
   % sufficies to show that
   % $\Vfil(\mixsigma)\leq max(\Vfil(\fwdprof), \Vfil(\difprof)$ when
   % the filter always forwards content upon receiving a clean signal
   % and randomizes otherwise.
   Let $\gamma_0$ and $\gamma_1$ be the filter's probability of
   blocking at each of its information sets.  Let
   $\tilde{\pi}_i(q(\mixstrfil))$ be the consumer's unique optimal
   information strategy for filter strategy $\mixstrfil$ and let

   \begin{align}
   \beta_{\gamma}&=q(\pi_0(1-\gamma_0) + (1-\pi_0)(1-\gamma_1)) +
                       (1-q)(\pi_1(1-\gamma_0) + (1-\pi_1)(1-\gamma_1)) \nonumber \\
                     &= q(\pi_0(1-\gamma_0) + (1-\pi_0)(1-\gamma_1))/q(\mixsigma) \nonumber
   \end{align}
   be the unconditional probability the filter forwards.  Then
   \begin{align}
     &\Vfil(\mixstrfil) = -c_1(1-q)(\pi_1(1-\gamma_0) + (1-\pi_1)(1-\gamma_1)) \;\; + \nonumber \\
     &\beta_{\gamma}\big( q(\mixstrfil)(1-\tilde{\pi}_0(q(\mixstrfil)))(-c_2) +(1-q(\mixstrfil))(\tilde{\pi}_1(q(\mixstrfil))(-c_1) + (1-\tilde{\pi}_1(q(\mixstrfil)))b)\big) \label{eq:misfilu}
   \end{align}
   It can be shown that the term inside the large parenthesis is
   linear in $q(\mixstrfil)$ when $\qL<q(\mixstrfil)<\qH$ and does not
   depend on $q(\mixstrfil)$ otherwise and therefore the entire term
   is linear in $\gamma$.  Therefore $\Vfil(\mixstrfil)$ is optmized
   when $\gamma_0, \gamma_1 \in \{0,1\}$ which corresponds to any of
   the four pure strategies and since $V(\fwdprof)$ and $V(\difprof)$
   are lower bounded by the other two profiles $\Vfil(\mixstrfil)$ is
   upper bounded by the maximum of $\Vfil(\fwdprof)$ and
   $\Vfil(\difprof)$.
 \end{proof}

 \begin{lem}
   \label{lem:linq}
   For a consumer optimal mixed profile $\mixsigma$ with filter
   strategy $\mixstrfil$ and consumer optimal information strategy
   $\tilde{\pi}_i$, if $\qL<q(\mixstrfil)<\qH$,  then $(1-\tilde{\pi}_0(q(\mixstrfil))
   q(\mixstrfil)$,$(1-\tilde{\pi}_1(q(\mixstrfil)) (1-q(\mixstrfil))$ and
   $\tilde{\pi}_1(q(\mixstrfil) (1-q(\mixstrfil))$  are all linear in
   $q(\mixstrfil)$ and have no other dependence on $\pi_0$ and $\pi_1$.
   \end{lem}

   \begin{proof}
     After tedious algebra it can be shown that
     \begin{align}
       (1-\tilde{\pi}_0(q(\mixstrfil))q(\mixstrfil) = \frac{e^{-c_2/\lambda}}{1-e^{-c_2/\lambda}}(q(\mixstrfil)-\qH) \nonumber \\
       \tilde{\pi}_1(q(\mixstrfil)(1-q(\mixstrfil)) = \frac{e^{-c_1/\lambda}}{e^{b/\lambda}-e^{c_1/\lambda}}(q(\mixstrfil)-\qL) \nonumber \\
       \tilde{\pi}_1(q(\mixstrfil)(1-q(\mixstrfil)) = \frac{e^{b/\lambda}}{e^{b/\lambda}-e^{c_1/\lambda}}(\qH-q(\mixstrfil)) \nonumber \\
     \end{align}
     which are all linear in $q(\mixstrfil)$.  Furthermore, $\pi_0$
     and $\pi_1$ only enter through $q(\mixstrfil)$.  
   \end{proof}

   \begin{proof}[Proof of Theorem ((VoT))]
     The consumer's VoT is the same as in the aligned case since for a
     fixed filter strategy, the consumer's optimal payoffs are the
     same as in the aligned case.  For the filter, VoT is trivially
     the same as in the aligned case except under $\difprof$ where
     $\qL<q(\strdif)<\qH$.  In that case, the filter's payoffs are given
     by equation \ref{eq:misfilu} with $\gamma_0=1$ and $\gamma_1=0$.
     By lemma \ref{lem:linq}, the term inside the parenthesis is
     linear in $q(\strdif)$ and since
     $\beta_{\gamma} = \frac{(1-\pi_0)q}{q(\strdif)} =
     \frac{(1-q)(1-\pi_1)}{1-q(\strdif)}$, the entire expression is linear
     in $\pi_0$ and $\pi_1$.  Furthermore,we can derive
     \begin{align}
     \frac{\partial \Vfil(q(\difprof))}{\partial \pi_0} =
       \frac{qe^{-c_1/\lambda}}{e^{b/\lambda}-e^{-c_1/\lambda}}\big((1-\qL)(b+c_1) -\qL c_2\big)
       \end{align}
       where the sign is determined by the term in the parenthesis,
       which is always positive since at $\qL$ it is optimal for the
       consumer to accept all content.  We can do the same for
       $\pi_1$:
         
     \begin{align}
     \frac{\partial \Vfil(q(\difprof))}{\partial \pi_1} =
       - \frac{1-q}{1-e^{-c_2/\lambda}}\big((1-\qL)(b+c_1) -\qL c_2\big)
       \end{align}
       where again the sign is determined by the term in the parenthesis,
       which is always positive by the same rationale as in the case of 
         $\pi_0$ and thus the entire term is negative.  
   \end{proof}

   % By lemma \ref{lem:cbr} the
   % consumer's best response to any mixed strategy is unique and thus
   % it's strategy is pure.    Therefore, any equilibrium
   % profile in which the filter blocks with positive probability at
   % both information sets achievs a payoff of $V(\blkprof)$.

   % Again let $\gamma_0$ and $\gamma_1$ be the
 %   filter's mixed probabilities of blocking at each of its information
 %   sets.  Then the filter's payoff can be written as
 %   \begin{align}
 %     \Vfil(\mixsigma) &= (1-q)(\pi_1(1-\gamma_0) + (1-\pi_1)(1-\gamma_1))(-c_1) + \beta_{\gamma}\big( q(\mixstrfil)(1-\tilde{\pi}_0)(-c_2) + (1-q(\mixstrfil))(\tilde{\pi}_1(-c_1) + (1-\tilde{\pi}_1)b)\big) \nonumber \\
 %     & = C +\alpha(\gamma_0) + \beta(\gamma_1) 
 %   \end{align}
 %   which is linear in $\gamma_0$ and $\gamma_1$.  Therefore, for it to be optimal
 %   for the filter to randomize a necessary condition is that
 %   $V(\mixsigma)$ be constant in $\gamma_0$ and $\gamma_1$ and thus
 %   $\alpha=\beta=0$.  This is only possible if $\tilde{\pi}_0=1$ and
 %   $\tilde{\pi}_1=-\frac{1-b}{b+c_1}$ which is imposible for any
 %   $-\frac{1-b}{b+c_1}\neq 1$ since lemma
 %   \ref{lem:cbr} establishes that if $\tilde{\pi}_0=1$, then
 %   $\tilde{\pi}_1=1$.  Therefore the only mixed strategy equilibrium
 %   can have $\tilde{\pi}_0=\tilde{\pi}_1=1$.  
 % \end{proof}

 \begin{proof}[Proof of Proposition \ref{prop:existsnoinfo}]
   Consider a consumer-optimal differentiating profile $\difprof$.
   For $\difprof$ to exist as an equilibrium, the detector must not
   have an incentive to deviate and forward all content while the
   consumer's strategy is held constant at.  Again let
   $\tilde{\pi}_i(q(\mixstrfil))$ be the consumer's optimal
   information choice when the filter plays a (possibly degenerate)
   mixed strategy This condition is given by:

    \begin{align}
      % &V(\sigma^d) - V(\sigma^t) >0 \nonumber \\
      % \text {where} \nonumber \\
      (1-q)\pi_1(-c_1) + \beta \bigg(q(\strdif)(1-\tilde{\pi}_0(\strdif))(-c_2) + (1-q(\strdif))\tilde{\pi}_1(\strdif)(-c_1) + (1-q(\strdif))(1-\tilde{\pi}_1(\strdif))b\bigg) >  \nonumber \\
      \bigg(-c_2 q(1-\tilde{\pi}_0(\strdif)) + -c_1(1-q)\tilde{\pi}_1(\strdif) +b(1-q)(1-\tilde{\pi}_1(\strdif))\bigg)
      \label{eq:devu}
    \end{align}
    % where the term in parentheses is the detector's utility from
    % deviating from a differentiating strategy, holding the user's
    % strategy constant at $\bar{s}_u$.  The expression for $V^*_d$ is
    % given by
    % \begin{align}
    %  V^*_d =  (1-q)\pi_2(-c_1) + \bigg(q(1-\pi_1) + (1-q)(1-\pi_2)\bigg)\
    %   \bigg(\tilde{q}(1-\tilde{\pi}_1)(-c_2) + (1-\tilde{q})\tilde{\pi}_2(-c_1) + (1-\tilde{q})(1-\pi_2)b\bigg)
    %   \label{eq:misequ}
        %       \end{align}
    where $\tilde{\pi}_0(\strdif)$ and $\tilde{\pi}_1(\strdif)$ are given in lemma \ref{lem:eqb}.  This is equivalent to
    \begin{align}
      \frac{\pi_0}{\pi_1} > \frac{1-q}{q}\bigg(\frac{1-\tilde{\pi}_1(\strdif)}{1-\tilde{\pi}_0(\strdif)}\bigg)\frac{b + c_1}{c_2}
    \end{align}   
    Substituting in the value for $\tilde{\pi}_0(\strdif)$ and $\tilde{\pi}_1(\strdif)$ and noting
    that $\frac{e^{b/\lambda}(1-e^{-c_2/\lambda})}{-e^{-c_2/\lambda} (e^{b/\lambda}-e^{-c_1/\lambda})}=\frac{1-\qL}{\qL}$
     yields the claimed result.
    Performing a similar calculation for $\fwdprof$ yields
    \begin{align}
      \frac{\pi_0}{\pi_1} < \frac{1-q}{q}\bigg(\frac{1-\tilde{\pi}_1(\strfwd)}{1-\tilde{\pi}_0(\strfwd)}\bigg)\frac{b + c_1}{c_2}
    \end{align}
    and making similar substitutions yields the result.

    Suppose that $\qL<q(\mixstrfil)<\qH$.
    A necessary condition for the existence of a mixed strategy
    equilibrium if for the filter to be indifferent between blocking
    and forwarding when it receives a signal that the content is
    malicious.

    Consider a consumer optimal mixed strategy profile $\mixsigma$
    with filter strategy $\mixstrfil$ that blocks with probability
    $\gamma$ after receiving the signal that content is malicious.
    Let $\hat{q}=\frac{\pi_0 q}{\pi_0q+\pi_1q}$ be the probability
    content is malicious given the filter received the malicious
    signal.  Then indifference requires
    \begin{align}
      (1-\hat{q})(-c_1) = \hat{q}(1-\tilde{\pi}_0(\mixstrfil))(-c_2) + (1-\hat{q})\tilde{\pi}_1(\mixstrfil)(-c_1) + (1-\hat{q})(1-\tilde{\pi}_1(\mixstrfil))b \nonumber \\
      \rightarrow \frac{1-\tilde{\pi}_0(\mixstrfil)}{1-\tilde{\pi}_1(\mixstrfil)}=\frac{1-\hat{q}}{\hat{q}}\frac{b+c_1}{c_2}
      \rightarrow \frac{\qL}{1-\qL}\frac{1-\pi_1\gamma}{1-\pi_0\gamma}\frac{1-q}{q}= \frac{\pi_1(1-q)}{\pi_0q}\frac{b+c_1}{c_2}
      \rightarrow \frac{b+c_1}{c_2}\frac{1-\qL}{\qL}=\frac{\pi_0(1-\pi_1\gamma)}{\pi_1(1-\pi_0\gamma)}
    \end{align}
    which for $\gamma \in  [0,1]$, it can only be satisfied when
    \begin{align}
      \frac{\pi_0}{\pi_1}<\frac{b+c_1}{c_2}\frac{1-\qL}{\qL}<\frac{1-\pi_1}{1-\pi_0}
    \end{align}
    This condition is also a sufficient condition for the filter to
    randomize since the filter's payoff after receiving each signal is
    lower bounded by the consumer's action payoff for each of the
    filter's signals.  Since the consumer does incur positive
    information costs and its payoff at the information set where the
    filter receives a malicious signal is less than $-c_1(1-\hat{q})$,
    the consumer's action payoff at the other information set must be
    greater than $-c_1(1-q(\strdif))$ (else it would not incur
    information costs and always block) and thus the filter does not
    have an incentive to block.

    If $q(\mixstrfil)< \qL$ no mixed strategy equilibrium
    exists since the filter's payoff when it receives a malicious
    signal is $(1-\hat{q})(\pi_1 (\gamma(-c_1) + (1-\gamma)b) +
    (1-\pi_1)b) -\hat{q}c_2(\pi_0(1-\gamma) + (1-\pi_1))$ which is
    linear and nonconstant in $\gamma$.  
  \end{proof}

%   \begin{proof}[Proof of Proposition \ref{prop:trans}]
%     A consumer would be willing to transfer $y$ units of utility to
%     switch from an equilibrium in which the filter never blocks to one
%     in which it differentiates as long as:
%     \begin{align}
%       R(\sigma^d) - \beta\lambda_{\texttt{c}} I(\sigma^d) - (R(\sigma^s)-\lambda_{\texttt{c}} I(\sigma^s))>y
%     \end{align}
%     Similarly, the amount, $y$, the filter would have to be paid ex-post to
%     commit to a differentiating strategy is given by
%     \begin{align}
%       y>R(\sigma^t) - R(\sigma^d)
%     \end{align}
% Rearranging terms gives the expression in proposition \ref{prop:trans}.
%   \end{proof}
  
  \section{Generalizations}

  In this section we generalize theorem \ref{thm:dvdp} to the case of
  general convex cost functions.

  Let $C(\mu;\tilde{q})$ be the consumer's cost for choosing
  information strategy $\mu$ when their prior belief that content is
  malicious is $\tilde{q}$.  Assume:
  \begin{enumerate}
  \item $C$ is strictly convex in $\mu$
  \item $C$ is strictly concave in $\tilde{q}$
  \item $ C$ is differentialble in $\mu$ and $\tilde{q}$
    \item $C(\mu;\tilde{q})=0$ if and only if
      $P(X|\Psi_{\texttt{c}})=P(X)$. 
    \end{enumerate}
    Items 1-3 are standard assumptions.  Item $4$ says that the
    consumer can costlessly choose to gather no information and any
    other information that shifts the distribution away from the prior
    must be costly.   

    Let $\vec{\tilde{q}} = [\tilde{q}, (1-\tilde{q})]^{\prime}$ and
    $\vec{\tilde{\Pi}}(\mu) = \begin{bmatrix}
\tilde{\pi}_1 & 1-\tilde{\pi}_1 \\
\tilde{\pi}_2 & 1-\tilde{\pi}_2
\end{bmatrix}$ and $\vec{R} = \begin{bmatrix} 0 & -c_1 \\c_2 & b\end{bmatrix}$

  Assume the filter plays a differentiating profile.
Then the consumer choose $\tilde{\pi_1}$ and $ \tilde{\pi_2}$ to optimize
\begin{equation}
  V_g((\bar{s}_{\texttt{f}}, s_{\texttt{c}}, \mu))=  tr\left(\vec{\tilde{\Pi}}(\mu)\vec{R}\right) \cdot \vec{\tilde{q}} - C(\mu; \tilde{q})
\end{equation}
Since the consumer's strategy space is compact and $V_g$ is a concave
function minus a convex function, the consumer has a unique optimal
choice of $\mu$.  The consumer incurs positive information costs if
and only if there exists a $\mu^{\prime}$ such that $C(\mu^{\prime},
\tilde{q})>0$ and $V_g((\bar{s}_{\texttt{f}}, s_{\texttt{c}},
\mu^{\prime})) > \max(-(1-\tilde{q})c_1, -\tilde{q}c_2 +
(1-\tilde{q}b))$.  For sufficiently high values of $c_1$ and $c_2$,
such a $\mu^{\prime}$ is guaranteed to exist.  Furthermore, it is
straightforward to show that for sufficiently high values of $\pi_1$
and low values of $\pi_2$ the filter's optimal strategy is to
differentiate.  We can now show that increasing the filter's quality
never reduces social optimality.  

\begin{prop}
  Assume there exists a $\mu^{\prime}$ such that $V_g((\bar{s}_{\texttt{f}}, s_{\texttt{c}},
\mu^{\prime})) > \max(-(1-\tilde{q})c_1, -\tilde{q}c_2 +
(1-\tilde{q}b))$ and the socially optimal strategy for the filter is
to play a differentiating strategy yielding payoffs $V(\sigma*)$.
Then:
\begin{enumerate}
\item $\frac{\partial V(\sigma^*)}{\partial \pi_1}>0$
  \item $\frac{\partial V(\sigma^*)}{\partial \pi_2}<0$
\end{enumerate}
\end{prop}

\begin{proof}
  To show $1$, we need to prove
  \begin{align}
    &\frac{\partial}{\partial \pi_1} \left((1-\pi_1)q + (1-\pi_2)(1-q)\right) \times \nonumber \\
    &\left( (1-\tilde{\pi}_1)\tilde{q}-c_2 + (1-\tilde{q})(\tilde{\pi}_2-c_1 + (1-\tilde{q})(1-\tilde{\pi}_2)b - C(\mu; \tilde{q})\right)>0 \nonumber 
  \end{align}
  This amounts to
  \begin{equation}
    A\left(\left(\frac{\partial Z}{\partial \tilde{\pi}_1} +
    \frac{\partial Z}{\partial \tilde{\pi}_2}\right) \times
  \left(\frac{\partial \tilde{\pi}_1}{\partial \tilde{q}} \frac{\partial \tilde{q}}{\partial \pi_1}\right) + \frac{\partial Z}{\partial\tilde{q}}\frac{\partial \tilde{q}}{\partial\pi_1}\right) + Zq
\label{eq:inc}
  \end{equation}
  where $A=\left((1-\pi_1)q + (1-\pi_2)(1-q)\right)$ and $Z=\left(
    (1-\tilde{\pi}_1)\tilde{q}(-c_2) + (1-\tilde{q})(\tilde{\pi}_2(-c_1) +
    (1-\tilde{q})(1-\tilde{\pi}_2)b + C(\mu; \tilde{q})\right)$.
  However, by enforcing optimality for the consumer $\frac{\partial Z}{\partial \tilde{\pi}_1}=
  \frac{\partial Z}{\partial \tilde{\pi}_2}=0$.  Therefore, equation
  \ref{eq:inc} simplifies to
  \begin{equation}
    (1-\tilde{\pi}_1)c_2 + (1-\tilde{q})\frac{\partial C}{\partial \tilde{q}} + C(\mu;\tilde{q})>0
    \label{eq:fin}
  \end{equation}
  By the definition of concavity (and notationally dropping the
  dependence on $\mu$), it must be that
  \begin{equation}
  C(\tilde{q}') - C(\tilde{q}) < \frac{\partial{C}}{\partial\tilde{q}}(\tilde{q}' - \tilde{q})
\end{equation}
for any $\tilde{q}$ and $\tilde{q}^{\prime}$. Plugging in $1$ for
$\tilde{q}^{\prime}$ and rearranging yields
\begin{equation}
  \frac{\partial{C}}{\partial\tilde{q}}(1 - \tilde{q}) +C(\tilde{q})>C(1)>0
  \end{equation}
which then implies that inequality \ref{eq:fin} is satisfied since the
first term is positive and the sum of the second and third term are
positive and this completes the proof.
  
\section{Attacker Proof Sketches}
This section is to be integrated, I just want to get the math typed up
so I don't forget.

\begin{prop}
  If $q_L<\tilde{q}<q_H$, the attacker's payoff is decreasing in
  $\nu$.
\end{prop}

\begin{proof}

  Suppose no filter
  \begin{align}
    V_a = \nu\left(1-\tilde{\pi_1}\right)
  \end{align}
  where $\tilde{\pi_1}$ is the equilibrium user attention when
  $\tilde{q}=\frac{nu}{1+\nu}$.  We can rewrite $V_a$ as
  \begin{align}
    V_a = (1+\nu)\tilde{q}\left(1-\tilde{\pi_1}\right)
  \end{align}
  Taking derivatives gives
  \begin{align}
    \frac{d V_a}{d \nu} = (1+\nu)\frac{d\tilde{q}}{d\nu}\frac{d}{d \tilde{q}}\left(\tilde{q}(1-\tilde{\pi_1})\right) + \tilde{q}(1-\tilde{\pi_1})
  \end{align}
  Since $\frac{d \tilde{q}}{d \nu} = \frac{1}{(1+\nu)^2}$ we have

  \begin{align}
    \frac{d V_a}{d \nu} = \frac{1}{1+\nu}\frac{d}{d \tilde{q}}\left(\tilde{q}(1-\tilde{\pi_1})\right) + \tilde{q}(1-\tilde{\pi_1})
  \end{align}

  However, it can be shown that $\frac{d}{d
    \tilde{q}}\left(\tilde{q}(1-\tilde{\pi_1})\right)$ is a constant
  and does not depend on $\tilde{q}$ or $\nu$.  Therefore, we have

  \begin{align}
    \frac{d V_a}{d \nu} = \frac{1}{1+\nu}C + \tilde{q}(1-\tilde{\pi_1})
  \end{align}
  where $C$ is some constant.  Now the second derivative is given by

  \begin{align}
    \frac{d^2 V_a}{d^2 \nu} = \frac{-1}{(1+\nu)^2}C + \frac{1}{(1+\nu)^2}C = 0
  \end{align}
  so the attacker's expected utility is linear.  We can use an
  identical second derivative argument to show that it is linear when
  there is a detector. 

Arbitrarily close to $q_L$ the attacker get's positive payoff.
However, was $\nu$ approaches the value such that $\tilde{q}=q_H$ the
value $\nu (1-\tilde{\pi}_1)$ approaches $0$ since $\nu$ approaches a
constant and the second term approaches 0.  Since it is linear and we
found two points with lower $\nu$ greater than higher $\nu$, it must
be decreasing.  

\end{proof}

\begin{prop}
  The defender's optimal strategy is thresholded by some $q$.
\end{prop}

\begin{proof}

  For $q<qL$ concave because linear. For middle region, linear as well
  (use the expression for expected payoff in appendix).  For high
  region, use second derivative of condition 2 (derived in mma but
  maybe can do it otherwise).  Need to also show differentiable
  (derivative at jump points ``line up'')

\end{proof}

\begin{prop}
  There is an equilibrium in which the filter differentiates and not
  an equilibrium where it doesn't if
  \begin{equation}
    \frac{b+c_1}{c_2}\frac{\pi_2}{\pi_1}<\frac{e^b/\lambda - e^{-c_1/\lambda}}{e^{c_2|}-1}
  \end{equation}
  or equivalently
  \begin{equation}
    \frac{b+c_1}{c_2} < \frac{\pi_1}{\pi_2}\frac{q_L}{1-q_L}
  \end{equation}
  
\end{prop}

Assuming the consumer incurs no information costs and accepts all, it
is better to have a filter if $\nu(-c2) + b < (1-pi_1)\nu(-c_2) +
\pi_2(-c_1)+(1-\pi_2)b$ for some value of $\nu$.  The value of $\nu$
that makes the defender indifferent is
$\frac{b+c_1}{c_2}\frac{\pi_2}{\pi_1}$.  The value of $\nu$ where a
consumer with no filter starts consuming information is
$\nu=q_L/(1-_qL) = \frac{e^b/\lambda -
  e^{-c_1/\lambda}}{e^{c_2|}-1}$.  That means the defender jumps
before not consuming information if the inequality is met.

\end{proof}

\begin{prop}
  $q=q_L$ when $\nu=q_L/(1-q_L)$.  Furthermore, $\tilde{q}=q_L$ if
  $\nu = \frac{1-\pi_2}{1-\pi_1}q_L/(1-q_L)$
\end{prop}

\begin{proof}
  Straightforward, just solve for $q$ and $\tilde{q}$ in terms of
  $\nu$.    
\end{proof}

\begin{prop}
  The defender is better off at the no filter case if
  \begin{equation}
    \frac{b+c_1}{c_2}>\frac{q_L}{1-q_L}
  \end{equation}
\end{prop}

\begin{proof}
  Plug in the possible equilibrium values of $\nu$ into the two
  payoffs and solve
\end{proof}

\begin{prop}
  A defender can do better if it had a worse filter if
  \begin{equation}
    \frac{q_L}{1-q_L}< \frac{b+c_1}{c_2}<\frac{\pi_1}{\pi_2}\frac{q_L}{1-q_L}
  \end{equation}
\end{prop}

\begin{proof}

  The preceeding shows where the equilibrium is a differentiating one
  but the defender would be better off it wasn't.  Since ofr
  sufficiently low values of $\frac{\pi_1}{\pi_2}$ the
  non-differentiating equilibrium will then exist,  the defender can
  do better off by reducing $\frac{\pi_1}{\pi_2}$.  
\end{proof}
